# Supplementary material for: NormGrad: Finding the Pixels that Matter for Training
Source: arXiv:1910.08823 source file (2019-10-19)
Supplement: Supplementary file 1 [file suppl.tex]

\clearpage
\section*{Supplementary Materials}\label{s:suppl}

As noted in the paper, our formulation uses the area constraint (line 426) that some of the authors introduced in a concurrent ICCV publication. We followed ICCV 2019 instructions and attached the publication here for the benefit of the reviewers. Please note that this is a minor part of our paper for which, naturally, we are not claiming novelty.

\begin{figure*}[h]
\centering
\includegraphics[width=1.\linewidth]{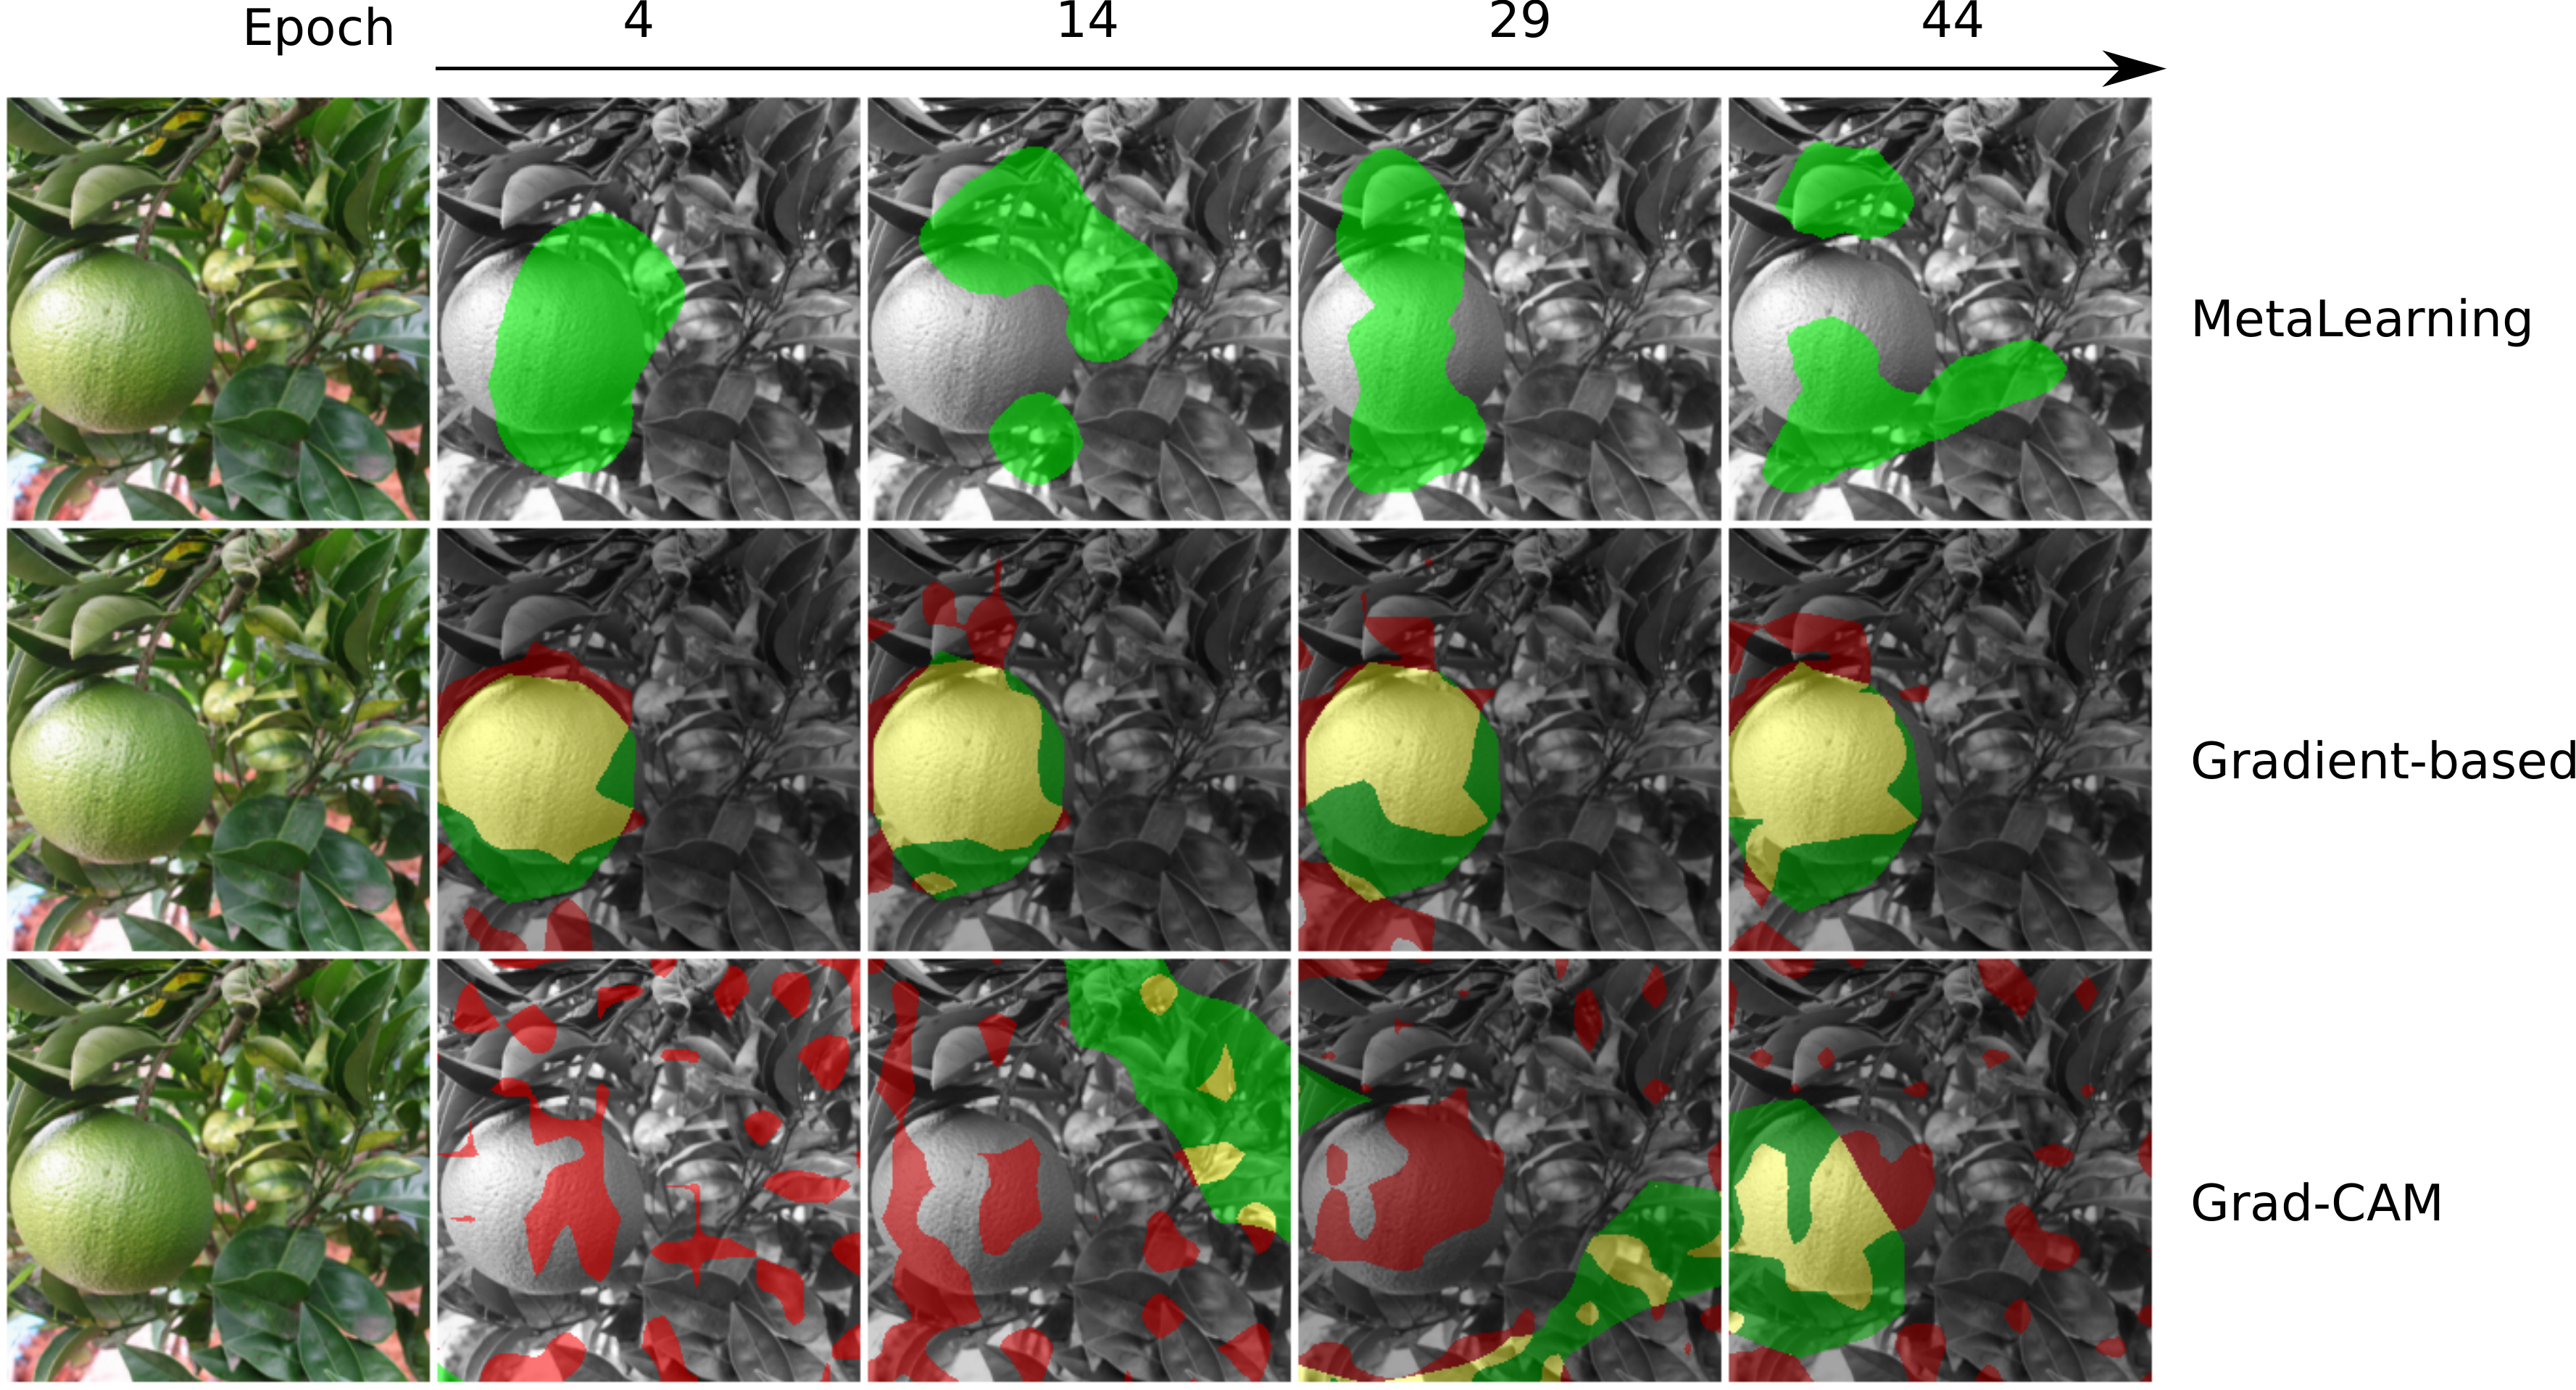}
\caption{\textbf{ImageNet image at resolution 224 $\times$ 224 .} We visualise the three methods at different training times and depths. The masks are colored according to their depth. For MetaLearning, we only use the full trainable network. For the other two methods, green denotes the fourth macro-block, red denotes the second macro-block, and yellow denotes areas common to both. Note how Grad-CAM is more appropriate for the end of the training (last on the right) and deeper representation (green + yellow). For different training times and depths, the gradient-based approach gives consistent masks fitting the objet. Finally, it is interesting to note how MetaLearning shifts its attention during training: from the object in the beginning to parts of the object and its surrounding (here the leaves) in the end. }
\label{fig:meta_vs_heuristic}
\end{figure*}

\clearpage
\includepdf[pages=-]{figures/fong19.pdf}
